# Supplementary material for: Unifying Top-down and Bottom-up Scanpath Prediction Using Transformers
Source: arXiv:2303.09383 source file (2024-03-30)
Supplement: Supplementary file 2 [file supp.tex]

% CVPR 2024 Paper Template; see https://github.com/cvpr-org/author-kit

\documentclass[11pt,twocolumn,letterpaper]{article}

%%%%%%%%% PAPER TYPE  - PLEASE UPDATE FOR FINAL VERSION
\usepackage{cvpr}              % To produce the CAMERA-READY version
% \usepackage[review]{cvpr}      % To produce the REVIEW version
% \usepackage[pagenumbers]{cvpr} % To force page numbers, e.g. for an arXiv version

% Import additional packages in the preamble file, before hyperref
\input{preamble}

% It is strongly recommended to use hyperref, especially for the review version.
% hyperref with option pagebackref eases the reviewers' job.
% Please disable hyperref *only* if you encounter grave issues, 
% e.g. with the file validation for the camera-ready version.
%
% If you comment hyperref and then uncomment it, you should delete *.aux before re-running LaTeX.
% (Or just hit 'q' on the first LaTeX run, let it finish, and you should be clear).
\definecolor{cvprblue}{rgb}{0.21,0.49,0.74}
\usepackage[pagebackref,breaklinks,colorlinks,citecolor=cvprblue]{hyperref}
\usepackage{algorithm}
\usepackage{algorithmic}
\usepackage{multirow}
\usepackage{csquotes}
\usepackage{color}% http://ctan.org/pkg/color
\usepackage{hyperref} 
\hypersetup{ 
 colorlinks=true, 
 linkcolor=black, 
 } 

% \usepackage[linkbordercolor={0 0 1}]{hyperref}

%%%%%%%%% PAPER ID  - PLEASE UPDATE
 % *** Enter the Paper ID here

%%%%%%%%% TITLE - PLEASE UPDATE
%\title{Unifying Top-down and Bottom-up Human Scanpath Prediction with Transformer}
\title{Unifying Top-down and Bottom-up Scanpath Prediction Using Transformers\\
\vspace{0.5em}{\it Supplementary Material}}
% Minh: I remove Human from the title. Should we put it back? 

%%%%%%%%% AUTHORS - PLEASE UPDATE
\author{Zhibo Yang\textsuperscript{1,2}, Sounak Mondal\textsuperscript{1}, Seoyoung Ahn\textsuperscript{1}, Ruoyu Xue\textsuperscript{1}, \\  Gregory Zelinsky\textsuperscript{1}, Minh Hoai\textsuperscript{1,3}, Dimitris Samaras\textsuperscript{1} \\
\textsuperscript{1}Stony Brook University~~~  \textsuperscript{2}Waymo LLC~~~
\textsuperscript{3}VinAI Research
}

\begin{document}
\input{definitions}
\maketitle
\tableofcontents
\clearpage
\setcounter{page}{1}
\maketitlesupplementary

\section{Rationale}
\label{sec:rationale}
Having the supplementary compiled together with the main paper means that:
\begin{itemize}
\item The supplementary can back-reference sections of the main paper, for example, we can refer to \cref{sec:intro};
\item The main paper can forward reference sub-sections within the supplementary explicitly (e.g. referring to a particular experiment); 
\item When submitted to arXiv, the supplementary will already included at the end of the paper.
\end{itemize}
To split the supplementary pages from the main paper, you can use \href{https://support.apple.com/en-ca/guide/preview/prvw11793/mac#:~:text=Delete%20a%20page%20from%20a,or%20choose%20Edit%20%3E%20Delete).}{Preview (on macOS)}, \href{https://www.adobe.com/acrobat/how-to/delete-pages-from-pdf.html#:~:text=Choose%20%E2%80%9CTools%E2%80%9D%20%3E%20%E2%80%9COrganize,or%20pages%20from%20the%20file.}{Adobe Acrobat} (on all OSs), as well as \href{https://superuser.com/questions/517986/is-it-possible-to-delete-some-pages-of-a-pdf-document}{command line tools}.
{
    \small
    \bibliographystyle{ieeenat_fullname}
    \bibliography{main}
}

\end{document}
